# Supplementary material for: NICGSlowDown: Evaluating the Efficiency Robustness of Neural Image Caption Generation Models
Source: arXiv:2203.15859 source file (2022-03-29)
Supplement: Supplementary file 1 [file appendix.tex]

\section{More Preliminary Results}
\label{sec:appendix_pre}
\begin{figure}[h]
    \centering
    \includegraphics[width=0.95\textwidth]{Figure/appendix_pre.pdf}
    \caption{How 3D dimension scaling affect FLOPs and latency on CPU devices.}
    \label{fig:appendix_pre}
\end{figure}

\figref{fig:appendix_pre} show how 3D dimension scaling affect the neural networks FLOPs and inference latency on CPU devices.
Similar with the results in \figref{fig:premilary}, the three-dimension scale would have different affect on these efficiency metrics. 
And the relationship between the neural networks dimension and these matrices are complex.

\section{More Experimental Setting}

\subsection{Description of Datasets}

CIFAR-10 dataset is drawn from the labeled subsets of the 80 million tiny images dataset.
The CIFAR-10 dataset consists of 60,000 color images in 10 classes, with 6000 images per class.
CIFAR-100 is similar to CIFAR-10 but with 100 classes, and each class contains 600 images.
Both the CIFAR-10 and CIFAR-100 datasets contain 50,000 training images and 10,000 testing images, with the image resolution $32\times 32$.
The SVHN dataset is a real-world image dataset obtained from house numbers in Google Street View images. The SVHN dataset contains 10 classes, with 73,257 images for training and 26,032 images for testing. Each image in SVHN has a resolution of $32 \times 32$
The Tiny ImageNet dataset is a subset of ImageNet images with 200 classes, each with 500 training and 50 testing images. The images in Tiny ImageNet are resized with the resolution $64\times 64$.
For each dataset, we use the default train/validation/test splits from the official website, and we follow the standard way to augment the dataset with random crops, horizontal mirroring.

% \subsection{Detail Base DNN Architecture}

\subsection{Hyperparameters Configuration}

The detailed hyperparameters for training the  models in \secref{sec:experimetn} are shown in Table \ref{tab:hyperparameter}. Notice for each model, \eg \tool or the selected baselines, we apply the same hyperparameter settings.

\input{Table/hyperparameters}

\subsection{Efficiency Metric Measurement}

\textbf{FLOPs.} To count the floating-point operations (FLOPs), we follow the setting in \cite{yu2018slimmable} and infer FLOPs with batch size 1. Specifically, we use the library \texttt{PyTorch-OpCounter} to count the FLOPs in the inference process.

\textbf{Parameters.} To count the number of the parameters of the model, we follow the setting in \cite{hou2020dynabert} and only count the parameters of the activated sub-networks.  We also use the library \texttt{PyTorch-OpCounter} to count the number of the parameters.

\textbf{Latency.} To evaluate the inference speed on different hardware devices, we follow ~\cite{hou2020dynabert}, and experiment on Nvidia 1080 Ti GPU and Intel Xeon E5-2660 CPU. We set the inference batch size as 1. For each hardware device, we use each model to infer 50 times and measure the average latency.

%  To evaluate the inference speed on GPU, we follow [4], and experiment on the QNLI training
% set with batch size 128 and sequence length 128. The numbers are the average running time of 100
% batches on an Nvidia K40 GPU. To evaluate the inference speed on CPU, we experiment on Kirin
% 810 A76 ARM CPU with batch size 1 and sequence length 128

\section{More Experimental Results}

\subsection{More Results on Comparison With Individually Trained DNNs}
\label{sec:appendix_oracle}

\input{Table/cifar100_oracle}

\input{Table/svhn_oracle}

\input{Table/tiny_oracle}

\tabref{tab:cifar100_oracle}, \ref{tab:svhn_oracle}, and \ref{tab:tiny_oracle} show the accuracy of \tool and individually trained base DNNs on CIFAR-100, SVHN, and Tiny ImageNet dataset.
The results in these tables are similar with the observations in \tabref{tab:cifar10_oracle}.
From the results, we could observe that \textit{(i)} the larger resolution doesn't always result in higher accuracy, \eg VGG16 on SVHN dataset, which implies there is data redundancy in this scenario.
\textit{(ii)} in most cases, the accuracy of the largest sub-networks of \tool is higher base DNNs, which implies our training method is beneficial to DNNs accuracy. We explain it as our training method would help the networks learn the dataset's invariant features.

\subsection{More Results on Single Efficiency  Constraints}
\label{sec:appendix_single}

\begin{figure*}[h]
    \centering
    \includegraphics[width=0.95\textwidth]{Figure/cifar100_single.pdf}
    \caption{Comparison of achievable accuracy under single efficiency constraint for CIFAR100.}
    \label{fig:cifar_100_efficency}
\end{figure*}

\begin{figure*}[t]
    \centering
    \includegraphics[width=0.95\textwidth]{Figure/SVHN_single.pdf}
    \caption{Comparison of achievable accuracy under single efficiency constraint for SVHN.}
    \label{fig:svhn_efficency}
\end{figure*}

\begin{figure*}[h]
    \centering
    \includegraphics[width=0.95\textwidth]{Figure/Tiny_single.pdf}
    \caption{Comparison of achievable accuracy under single efficiency constraint for Tiny ImageNet.}
    \label{fig:tin_efficency}
\end{figure*}

\figref{fig:cifar_100_efficency}, \ref{fig:svhn_efficency}, and \ref{fig:tin_efficency} show the comparison of achievable accuracy under single efficiency for CIFAR-100,SVHN and Tiny ImageNet.
The results in these figures are similar with the results in \figref{fig:cifar_10_efficency}.
\tool could achieve the best performance under different constraints, with the same constraints, the accuracy of \tool is better than comparison baselines a significant margin.

\subsection{More Results on Multiple  Constraints}
\label{sec:appendix_multiple}

\begin{figure}[h]
    \centering
    \includegraphics[width=0.96\textwidth]{Figure/appendix_multpile.pdf}
    \caption{Comparison of model accuracy under the constraints of both FLOPs and Parameters for CIFAR100, SVHN and Tiny ImageNet.}
    \label{fig:appendix_multpile}
\end{figure}

\figref{fig:appendix_multpile} show the model accuracy under the constraints of both FLOPs and Parameters for CIFAR100, SVHN and Tiny ImageNet. The results in \figref{fig:appendix_multpile} is simliar with the results in \figref{fig:multiple}. With multiple constraints, there exist computational resource waste in the selected baseline, but \tool could make use of the computational resource to achieve better accuracy.
For example, The depth-adaptive method ~(the rectangle point) is better in saving FLOPs than width-adaptive methods but performing poorly in balancing accuracy and number of parameters.
Because \tool could scale both depth and width direction, \tool could perform better under multiple constraints.
